# Supplementary material for: Spin-orbit-enhanced magnetic surface second-harmonic generation in Sr$_2$IrO$_4$
Source: arXiv:2011.11662 source file (2020-11-23)
Supplement: Supplementary file 1 [file supplement.pdf]

# Supplemental Material:
# Spin-orbit-enhanced magnetic surface second-harmonic generation in $Sr_2IrO_4$

K. L. Seyler, A. de la Torre, Z. Porter, E. Zoghlin, R. Polski, M. Nguyen, S. Nadj-Perge, S. D. Wilson, and D. Hsieh

**Contents**

I. Experimental methods 2

II. Absence of laser-induced magnetic rearrangement 3

III. Fitting the zero-field RA data 4

IV. Fitting the high-field RA data 5

V. $\beta$ dependence of the anomalous $C_1$ term 8

VI. Fitting RA data by scaling the MD contribution 9

VII. SHG evidence for $a$-$b$ symmetry breaking and twinning 10

References 12

## I. Experimental methods

Single crystals of $Sr_2IrO_4$ were grown using an established flux method [1]. Dry starting powders of $SrCO_3$, $IrO_2$, and anhydrous $SrCl_2$ were placed in a 2:1:5.5 molar ratio within a 100 mL Pt crucible with a lid. The crucible was slowly heated to 1370 °C in air, soaked for 5 hours, cooled to 850 °C at 6 °C per hour, and then furnace-cooled to room temperature. Single crystals were then obtained by dissolving the excess flux in deionized water. Magnetization data were collected on a cleaved and polished sample mounted on a quartz paddle with GE varnish, and measured with a Quantum Design MPMS3 system in the vibrating sample magnetometer mode. Samples for SHG were affixed to an oxygen-free high thermal conductivity copper mount using a small amount of Torr seal on the underside of the sample, then cleaved along the (001) face prior to measurement and pumped down below $10^{-7}$ torr in a continuous flow optical cryostat. The crystal orientation was checked by x-ray diffraction. We found consistent results for the SHG magnetic field dependence across multiple samples. We note that the essential features of the zero-field SHG, namely, the presence of a $C_1$ term that onsets below ∼230 K, agree with prior reports [2]. However, the RA patterns differ in the relative magnitude of adjacent lobes in the $S_{\text{out}}$ geometries and the rotation away from the high symmetry directions for EQ SHG, which are markers of mirror symmetry breaking. These differences may stem from the high sensitivity of $Sr_2IrO_4$ to slight variations in growth conditions [3]. The data presented here are representative of samples grown by the methods in Ref. [1].

RA-SHG measurements were performed using a rotating scattering plane technique [4] with 100 fs laser pulses at 800 nm from a Ti:sapphire amplifier (100 kHz repetition rate). A schematic of the experimental geometry is shown in Fig. S1. The fluence was fixed at 2 mJ/cm$^2$ with an angle of incidence of $\theta = 10°$, except for the low-fluence Ti:sapphire oscillator measurements in Fig. S2(a), which used 10 µJ/cm$^2$. In-plane magnetic fields were applied using SmCo permanent magnets placed adjacent to the sample in a home-built rotator apparatus [Fig. S1], which allows for free rotation of the magnets about the cylindrical sample holder. The rotator can house several 3/8” × 3/8” × 1/8” SmCo magnets ($T_C \sim 1000$ K), with field strength adjustable by changing the number of magnets and their spacing. The magnetic field strengths were measured at room temperature with a gauss meter, and we assume constant magnetic field within our 80 K to 300 K range. The maximum field we achieved with SmCo magnets was 370 mT. The in-plane field direction is manually tunable using permanent magnets fixed to the outside rim of the cryostat. Wide-field SHG imaging was performed at $\theta \sim 3°$ with a fluence of 4 mJ/cm$^2$ in $P_{\text{in}}$-$P_{\text{out}}$ geometry.

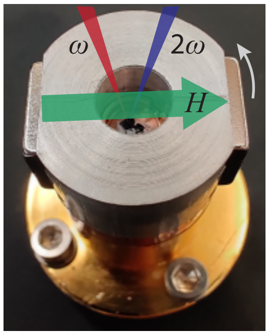


FIG. S1. Image of the home-built magnet rotator setup. A cylindrical copper sample mount holds an aluminum ring in place and allows for free rotation of the magnets about the cylinder axis.

## II. Absence of laser-induced magnetic rearrangement

We examined the possibility that the SHG onset ∼230 K in $Sr_2IrO_4$ is due to a metastable magnetic order induced by high-field laser pulses as suggested in Ref. [5]. To do so, we cleaved a fresh (not previously irradiated) $Sr_2IrO_4$ sample and measured the temperature-dependent SHG intensity at a fluence of ∼10 µJ/cm$^2$, 200 times lower than that used for the data shown in the main text, using a Ti:sapphire oscillator. To achieve sufficient signal-to-noise, we used 20 min integration times and pixel binning with an electron-multiplying charge-coupled device at a single angle of incidence where the intensity was at a maximum. Figure S2(a) shows that the SHG onset below ∼230 K is still clearly present. A laser-induced metastable stacking re-arrangement is therefore an unlikely explanation for the anomalous $C_1$ SHG term.

To rule out the possibility of a transient laser-induced effect, we performed an ultrafast pump-probe SHG experiment at 80 K to track the temporal change in SHG intensity following a pump pulse. Figure S2(b) shows a typical SHG transient in $P_{\rm in}$-$S_{\rm out}$ geometry using a ∼100 fs pump at 1400 nm with a fluence of 360 µJ/cm$^2$ from an optical parametric amplifier. We observe an ultrafast suppression rather than enhancement of the SHG intensity after the pump pulse, which rules out any possibility that the enhanced SHG intensity below $T_N$ is due to a laser-induced effect on the timescale of the laser pulse.

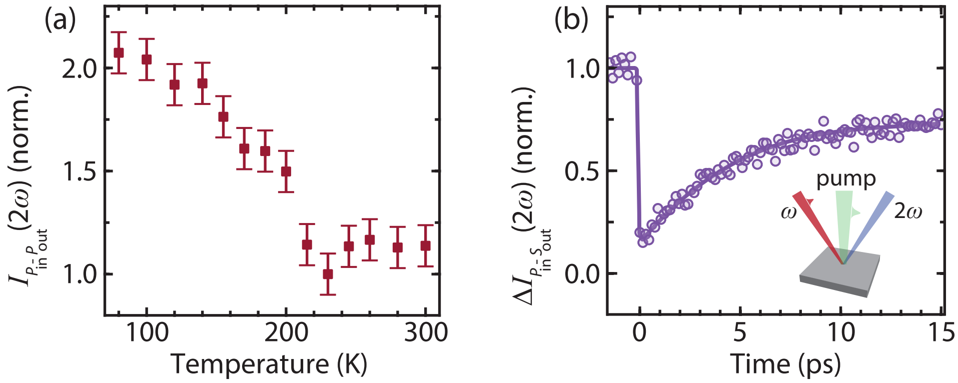


FIG. S2. (a) SHG intensity from a freshly cleaved $Sr_2IrO_4$ sample, taken under $P_{\rm in}$-$P_{\rm out}$ geometry at the $\phi$ of maximum intensity and normalized by its room-temperature value. The error bars represent the standard deviation over six independent measurements at the same temperature. (b) Change in SHG intensity as a function of time delay after the pump pulse at 80 K. The data is measured at the $\phi$ that gives maximum SH intensity for $P_{\rm in}$-$S_{\rm out}$. Solid line is a guide to the eye. Inset shows a schematic of the experimental geometry with a normally incident pump and oblique probe beam.

### III. Fitting the zero-field RA data

Below $T_N$ in zero magnetic field, the RA patterns can be described by the square of a coherent sum of a bulk EQ term respecting the $4/m$ crystallographic point group and a surface ED term arising from the surface magnetic point group, $2'$. The second-harmonic polarizations for the EQ and ED terms are respectively expressed as $P_i(2\omega) \propto \chi^{\mathrm{EQ}(i)}_{ijkl} E_j(\omega)\partial_k E_l(\omega)$ and $P_i(2\omega) \propto \chi^{\mathrm{ED}(c)}_{\mathrm{s},ijk} E_j(\omega)E_k(\omega)$, where $E(\omega)$ is the fundamental electric field at frequency $\omega$, and $\chi^{\mathrm{EQ}(i)}_{ijkl}$ and $\chi^{\mathrm{ED}(c)}_{\mathrm{s},ijk}$ are the $i$-type bulk EQ and $c$-type surface ED susceptibility tensors. The total SHG intensity is given by

$$I(2\omega, \phi) = |A_{\mathrm{EQ}} \hat{e}^{\mathrm{out}}_i \chi^{\mathrm{EQ}(i)}_{ijkl} \hat{e}^{\mathrm{in}}_j q_k \hat{e}^{\mathrm{in}}_l + A_{\mathrm{ED}} \hat{e}^{\mathrm{out}}_i \chi^{\mathrm{ED}(c)}_{\mathrm{s},ijk} \hat{e}^{\mathrm{in}}_j \hat{e}^{\mathrm{in}}_k|^2 I(\omega)^2, \tag{1}$$

where $\vec{q}$ is the wavevector of incident light, $\hat{e}$ is the polarization of incoming fundamental or outgoing second-harmonic light, $I(\omega)$ is the intensity of fundamental beam, and $A_{\mathrm{EQ}}$ and $A_{\mathrm{ED}}$ are constants. The expressions for the $4/m$ EQ term have been thoroughly detailed in Ref. [6]. The third-rank polar $c$-tensor for the $2'$ ED SHG process has the form [7]

$$\chi^{\mathrm{ED}(c)}_{\mathrm{s},ijk} = \begin{pmatrix} \begin{pmatrix} \chi_{\mathrm{s},xxx} \\ \chi_{\mathrm{s},xxy} \\ 0 \end{pmatrix} & \begin{pmatrix} \chi_{\mathrm{s},xxy} \\ \chi_{\mathrm{s},xyy} \\ 0 \end{pmatrix} & \begin{pmatrix} 0 \\ 0 \\ \chi_{\mathrm{s},xzz} \end{pmatrix} \\ \begin{pmatrix} \chi_{\mathrm{s},yxx} \\ \chi_{\mathrm{s},yyx} \\ 0 \end{pmatrix} & \begin{pmatrix} \chi_{\mathrm{s},yyx} \\ \chi_{\mathrm{s},yyy} \\ 0 \end{pmatrix} & \begin{pmatrix} 0 \\ 0 \\ \chi_{\mathrm{s},yzz} \end{pmatrix} \\ \begin{pmatrix} 0 \\ 0 \\ \chi_{\mathrm{s},zzx} \end{pmatrix} & \begin{pmatrix} 0 \\ 0 \\ \chi_{\mathrm{s},zzy} \end{pmatrix} & \begin{pmatrix} \chi_{\mathrm{s},zzx} \\ \chi_{\mathrm{s},zzy} \\ 0 \end{pmatrix} \end{pmatrix}. \tag{2}$$

The ED contribution to the SH electric fields are therefore as follows:

$$\begin{aligned} E^{\mathrm{ED}}_{pp}(2\omega) \sim\ & \cos\theta \sin^2\theta((\chi_{\mathrm{s},xzz} + 2\chi_{\mathrm{s},zzx})\cos\phi - (\chi_{\mathrm{s},yzz} + 2\chi_{\mathrm{s},zzy})\sin\phi) \\ & + \cos^3\theta(\chi_{\mathrm{s},xxx}\cos^3\phi - (2\chi_{\mathrm{s},xxy} + \chi_{\mathrm{s},yxx})\cos^2\phi\sin\phi + (\chi_{\mathrm{s},xyy} + 2\chi_{\mathrm{s},yyx})\cos\phi\sin^2\phi - \chi_{\mathrm{s},yyy}\sin^3\phi) \end{aligned} \tag{3}$$

$$E^{\mathrm{ED}}_{sp}(2\omega) \sim \cos\theta(\chi_{\mathrm{s},xyy}\cos^3\phi + (2\chi_{\mathrm{s},xxy} - \chi_{\mathrm{s},yyy})\cos^2\phi\sin\phi + (\chi_{\mathrm{s},xxx} - 2\chi_{\mathrm{s},yyx})\cos\phi\sin^2\phi - \chi_{\mathrm{s},yxx}\sin^3\phi) \tag{4}$$

$$\begin{aligned} E^{\mathrm{ED}}_{ps}(2\omega) \sim\ & \sin^2\theta(\chi_{\mathrm{s},yzz}\cos\phi + \chi_{\mathrm{s},xzz}\sin\phi) \\ & + \cos^2\theta(\chi_{\mathrm{s},yxx}\cos^3\phi + (\chi_{\mathrm{s},xxx} - 2\chi_{\mathrm{s},yyx})\cos^2\phi\sin\phi + (-2\chi_{\mathrm{s},xxy} + \chi_{\mathrm{s},yyy})\cos\phi\sin^2\phi - \chi_{\mathrm{s},xyy}\sin^3\phi) \end{aligned} \tag{5}$$

$$E^{\mathrm{ED}}_{ss}(2\omega) \sim \chi_{\mathrm{s},yyy}\cos^3\phi + (\chi_{\mathrm{s},xyy} + 2\chi_{\mathrm{s},yyx})\cos^2\phi\sin\phi + (2\chi_{\mathrm{s},xxy} + \chi_{\mathrm{s},yxx})\cos\phi\sin^2\phi + \chi_{\mathrm{s},xxx}\sin^3\phi. \tag{6}$$

Using Eq. (1), we achieve good fits to the $P_{\mathrm{in}}$-$S_{\mathrm{out}}$ RA patterns, as shown in Fig. 1(c) inset and Fig. 4(b). Fits to the other polarization geometries are shown in Fig. S4. In general, the components of the ED nonlinear susceptibility tensor in Eq. (2) will depend on the surface magnetization, $\mathbf{M}_{\mathrm{s}}$, as shown explicitly in the following section.

## IV. Fitting the high-field RA data

In this section, we detail how the magnetization influences the second-harmonic response in $Sr_2IrO_4$, following the general framework laid out by Ref. [8] and Ref. [9]. Above the metamagnetic transition ($\sim$200 mT), $Sr_2IrO_4$ transitions from the $-++-$ ground state (magnetic point group $2/m1'$) into the ferromagnetic $++++$ state (magnetic point group $2'/m'$) [10]. In the $++++$ state, there are three SHG contributions: bulk EQ and surface ED as described above in Section III, and a new magnetization-dependent MD process

$$P_i(2\omega) \propto \chi^{\mathrm{MD(c)}}_{ijk}(\mathbf{M})E_j(\omega)H_k(\omega). \tag{7}$$

We note that the MD process $M_i(2\omega) \propto \chi^{\mathrm{MD}(c)}_{ijk}E_j(\omega)E_k(\omega)$ is also allowed, where $M_i(2\omega)$ is the second-harmonic nonlinear magnetization of the sample, but our data does not allow us to draw a distinction between this process and that of Eq. (7).

The total SHG intensity in the $++++$ state is given by

$$I(2\omega,\phi) = |A_{\mathrm{EQ}}\hat{e}^{\mathrm{out}}_i\chi^{\mathrm{EQ}(i)}_{ijkl}\hat{e}^{\mathrm{in}}_j q_k \hat{e}^{\mathrm{in}}_l + A_{\mathrm{ED}}\hat{e}^{\mathrm{out}}_i\chi^{\mathrm{ED}(c)}_{\mathrm{s},ijk}(\mathbf{M}_{\mathrm{s}})\hat{e}^{\mathrm{in}}_j\hat{e}^{\mathrm{in}}_k + A_{\mathrm{MD}}\hat{e}^{\mathrm{out}}_i\chi^{\mathrm{MD}(c)}_{ijk}(\mathbf{M})\hat{e}^{\mathrm{in}}_j\epsilon_{klm}q_l\hat{e}^{\mathrm{in}}_m|^2 I(\omega)^2, \tag{8}$$

where $\mathbf{M}$ ($\mathbf{M}_{\mathrm{s}}$) is the static bulk (surface) magnetization, $A_{\mathrm{MD}}$ is a constant, and $\epsilon_{klm}$ is the Levi-Civita symbol. The magnetization-dependent nonlinear susceptibility tensors may be expanded as $\chi_{ijk}(\mathbf{M}) = \chi_{0,ijk} + \chi_{ijkl}M_l$, where we omit terms that are nonlinear in the magnetization. $\chi_{0,ijk}$ represents the magnetization-independent crystallographic contribution, which is a third-rank axial (polar) tensor for the MD (surface ED) process [6]. These processes give $\phi$-independent terms in the SHG intensity, which are neglected because they cannot explain the high-temperature SHG patterns and they are not necessary for the fits [6]. In the MD (surface ED) case, we write $\chi_{ijkl}$ as $\chi^{\mathrm{MD}(i)}_{ijkl}$ ($\chi^{\mathrm{ED}(i)}_{\mathrm{s},ijkl}$), which is a fourth-rank polar (axial) tensor that respects the high-temperature crystallographic point group. Due to broken $a$-$b$ symmetry, we must assume either orthorhombic or monoclinic symmetry for $\chi^{\mathrm{MD}(i)}_{ijkl}$ and $\chi^{\mathrm{ED}(i)}_{\mathrm{s},ijkl}$. Under monoclinic symmetry [7],

$$\chi^{\mathrm{MD}(i)}_{ijkl} = \begin{pmatrix} \begin{pmatrix} \chi_{xxxx} & \chi_{xxxy} & 0 \\ \chi_{xxyx} & \chi_{xxyy} & 0 \\ 0 & 0 & \chi_{xxzz} \end{pmatrix} & \begin{pmatrix} \chi_{xyxx} & \chi_{xyxy} & 0 \\ \chi_{xyyx} & \chi_{xyyy} & 0 \\ 0 & 0 & \chi_{xyzz} \end{pmatrix} & \begin{pmatrix} 0 & 0 & \chi_{xzxz} \\ 0 & 0 & \chi_{xzyz} \\ \chi_{xzzx} & \chi_{xzzy} & 0 \end{pmatrix} \\ \begin{pmatrix} \chi_{yxxx} & \chi_{yxxy} & 0 \\ \chi_{yxyx} & \chi_{yxyy} & 0 \\ 0 & 0 & \chi_{yxzz} \end{pmatrix} & \begin{pmatrix} \chi_{yyxx} & \chi_{yyxy} & 0 \\ \chi_{yyyx} & \chi_{yyyy} & 0 \\ 0 & 0 & \chi_{yyzz} \end{pmatrix} & \begin{pmatrix} 0 & 0 & \chi_{yzxz} \\ 0 & 0 & \chi_{yzyz} \\ \chi_{yzzx} & \chi_{yzzy} & 0 \end{pmatrix} \\ \begin{pmatrix} 0 & 0 & \chi_{zxxz} \\ 0 & 0 & \chi_{zxyz} \\ \chi_{zxzx} & \chi_{zxzy} & 0 \end{pmatrix} & \begin{pmatrix} 0 & 0 & \chi_{zyxz} \\ 0 & 0 & \chi_{zyyz} \\ \chi_{zyzx} & \chi_{zyzy} & 0 \end{pmatrix} & \begin{pmatrix} \chi_{zzxx} & \chi_{zzxy} & 0 \\ \chi_{zzyx} & \chi_{zzyy} & 0 \\ 0 & 0 & \chi_{zzzz} \end{pmatrix} \end{pmatrix}. \tag{9}$$

In our experiments, we apply an in-plane magnetic field that creates a static in-plane magnetization $\mathbf{M} = (M_x, M_y, 0)$,

and leads to the third-rank axial $c$-tensor

$$\chi_{ijk}^{\mathrm{MD}(c)}(\mathbf{M}) = \begin{pmatrix} \begin{pmatrix} M_x\chi_{xxxx} + M_y\chi_{xxxy} \\ M_x\chi_{xxyx} + M_y\chi_{xxyy} \\ 0 \end{pmatrix} & \begin{pmatrix} M_x\chi_{xyxx} + M_y\chi_{xyxy} \\ M_x\chi_{xyyx} + M_y\chi_{xyyy} \\ 0 \end{pmatrix} & \begin{pmatrix} 0 \\ 0 \\ M_x\chi_{xzzx} + M_y\chi_{xzzy} \end{pmatrix} \\ \begin{pmatrix} M_x\chi_{yxxx} + M_y\chi_{yxxy} \\ M_x\chi_{yxyx} + M_y\chi_{yxyy} \\ 0 \end{pmatrix} & \begin{pmatrix} M_x\chi_{yyxx} + M_y\chi_{yyxy} \\ M_x\chi_{yyyx} + M_y\chi_{yyyy} \\ 0 \end{pmatrix} & \begin{pmatrix} 0 \\ 0 \\ M_x\chi_{yzzx} + M_y\chi_{yzzy} \end{pmatrix} \\ \begin{pmatrix} 0 \\ 0 \\ M_x\chi_{zxzx} + M_y\chi_{zxzy} \end{pmatrix} & \begin{pmatrix} 0 \\ 0 \\ M_x\chi_{zyzx} + M_y\chi_{zyzy} \end{pmatrix} & \begin{pmatrix} M_x\chi_{zzxx} + M_y\chi_{zzxy} \\ M_x\chi_{zzyx} + M_y\chi_{zzyy} \\ 0 \end{pmatrix} \end{pmatrix}. \tag{10}$$

The MD contributions to the SH electric fields are then given by

$$\begin{aligned} E_{pp}^{\mathrm{MD}}(2\omega) \sim\ & -\sin^2\theta(\chi_{zyz}\cos\phi + \chi_{zxz}\sin\phi) \\ & \cos^2\theta(-\chi_{xyx}\cos^3\phi + (-\chi_{xxx} + \chi_{xyy} + \chi_{yxx})\cos^2\phi\sin\phi + (\chi_{xxy} + \chi_{yxx} - \chi_{yyy})\cos\phi\sin^2\phi - \chi_{yxy}\sin^3\phi) \end{aligned} \tag{11}$$

$$\begin{aligned} E_{sp}^{\mathrm{MD}}(2\omega) \sim\ & \sin^2\theta(\chi_{zzy}\cos\phi + \chi_{zzx}\sin\phi) \\ & + \cos^2\theta(\chi_{xxy}\cos^3\phi + (\chi_{xxx} - \chi_{xyy} - \chi_{yxy})\cos^2\phi\sin\phi + (-\chi_{xyx} - \chi_{yxx} + \chi_{yyy})\cos\phi\sin^2\phi + \chi_{yyx}\sin^3\phi) \end{aligned} \tag{12}$$

$$E_{ps}^{\mathrm{MD}}(2\omega) \sim -\cos\theta(\chi_{yyx}\cos^3\phi + (\chi_{xyx} + \chi_{yxx} - \chi_{yyy})\cos^2\phi\sin\phi + (\chi_{xxx} - \chi_{xyy} - \chi_{yxy})\cos\phi\sin^2\phi - \chi_{xxy}\sin^3\phi) \tag{13}$$

$$E_{ss}^{\mathrm{MD}}(2\omega) \sim \cos\theta(\chi_{yxy}\cos^3\phi + (\chi_{xxy} + \chi_{yxx} - \chi_{yyy})\cos^2\phi\sin\phi + (\chi_{xxx} - \chi_{xyy} - \chi_{yyx})\cos\phi\sin^2\phi - \chi_{xyx}\sin^3\phi). \tag{14}$$

In the expressions above, $\chi_{ijk} = M_x\chi_{ijkx} + M_y\chi_{ijky}$. A similar exercise can be performed for the surface ED case, giving the third-rank polar $c$-tensor

$$\chi_{s,ijk}^{\mathrm{ED}(c)}(\mathbf{M}_{\mathrm{s}}) = \begin{pmatrix} \begin{pmatrix} M_{\mathrm{s},x}\chi_{\mathrm{s},xxxx} + M_{\mathrm{s},y}\chi_{\mathrm{s},xxxy} \\ M_{\mathrm{s},x}\chi_{\mathrm{s},xxyx} + M_{\mathrm{s},y}\chi_{\mathrm{s},xxyy} \\ 0 \end{pmatrix} & \begin{pmatrix} M_{\mathrm{s},x}\chi_{\mathrm{s},xxyx} + M_{\mathrm{s},y}\chi_{\mathrm{s},xxyy} \\ M_{\mathrm{s},x}\chi_{\mathrm{s},xyyx} + M_{\mathrm{s},y}\chi_{\mathrm{s},xyyy} \\ 0 \end{pmatrix} & \begin{pmatrix} 0 \\ 0 \\ M_{\mathrm{s},x}\chi_{\mathrm{s},xzzx} + M_{\mathrm{s},y}\chi_{\mathrm{s},xzzy} \end{pmatrix} \\ \begin{pmatrix} M_{\mathrm{s},x}\chi_{\mathrm{s},yxxx} + M_{\mathrm{s},y}\chi_{\mathrm{s},yxxy} \\ M_{\mathrm{s},x}\chi_{\mathrm{s},yyxx} + M_{\mathrm{s},y}\chi_{\mathrm{s},yyxy} \\ 0 \end{pmatrix} & \begin{pmatrix} M_{\mathrm{s},x}\chi_{\mathrm{s},yyxx} + M_{\mathrm{s},y}\chi_{\mathrm{s},yyxy} \\ M_{\mathrm{s},x}\chi_{\mathrm{s},yyyx} + M_{\mathrm{s},y}\chi_{\mathrm{s},yyyy} \\ 0 \end{pmatrix} & \begin{pmatrix} 0 \\ 0 \\ M_{\mathrm{s},x}\chi_{\mathrm{s},yzzx} + M_{\mathrm{s},y}\chi_{\mathrm{s},yzzy} \end{pmatrix} \\ \begin{pmatrix} 0 \\ 0 \\ M_{\mathrm{s},x}\chi_{\mathrm{s},zzxx} + M_{\mathrm{s},y}\chi_{\mathrm{s},zzxy} \end{pmatrix} & \begin{pmatrix} 0 \\ 0 \\ M_{\mathrm{s},x}\chi_{\mathrm{s},zzyx} + M_{\mathrm{s},y}\chi_{\mathrm{s},zzyy} \end{pmatrix} & \begin{pmatrix} M_{\mathrm{s},x}\chi_{\mathrm{s},zzxx} + M_{\mathrm{s},y}\chi_{\mathrm{s},zzxy} \\ M_{\mathrm{s},x}\chi_{\mathrm{s},zzyx} + M_{\mathrm{s},y}\chi_{\mathrm{s},zzyy} \\ 0 \end{pmatrix} \end{pmatrix}. \tag{15}$$

These tensor elements can be inserted into Eq. (3)–(6) to get the full surface-magnetization-dependent ED second-harmonic electric field expressions.

In Fig. 2(a) and Fig. S3, we display RA-SHG plots under an applied in-plane magnetic field of 0.37 T with varying field direction, $\beta$. Using Eq. (8), we achieve good simultaneous fits (as shown by the solid black lines) for each polarization geometry by only varying $\beta$ and assuming constant bulk and surface magnetization magnitudes,

$M_0$ and $M_{s,0}$, that both rotate with the field direction, $M_x = M_0 \cos\beta$, $M_y = M_0 \sin\beta$, $M_{s,x} = M_{s,0} \cos\beta$, and $M_{s,y} = M_{s,0} \sin\beta$. The clear pattern differences for $\beta = 0°$ and $\beta = 90°$ qualitatively show that tetragonal symmetry is broken. One must assume symmetry reductions to monoclinic or orthorhombic point groups to fit the data.

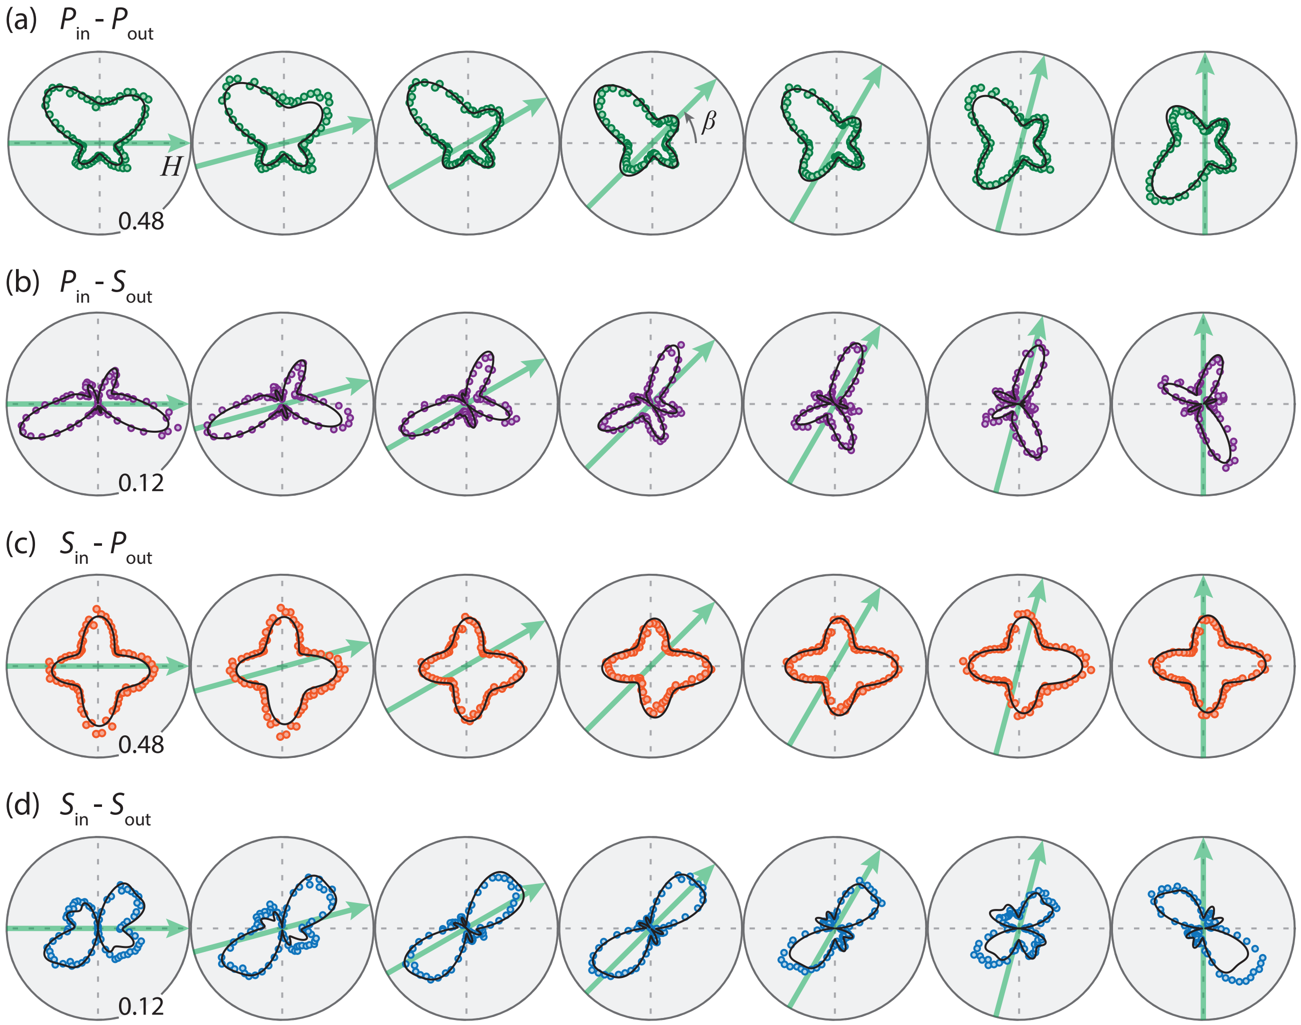


FIG. S3. RA-SHG intensity patterns for (a) $P_{\rm in}$-$P_{\rm out}$, (b) $P_{\rm in}$-$S_{\rm out}$, (c) $S_{\rm in}$-$P_{\rm out}$, and (d) $S_{\rm in}$-$S_{\rm out}$ measured at different applied magnetic field angles $\beta$, shown by the green arrows, with fixed field strength of 0.37 T at 80 K. The plots are presented in field angle increments of 15°. Solid black lines give fits with the theoretical model described in the text.

## V. $\beta$ dependence of the anomalous $C_1$ term

In Fig. 2(b), we show the summation of the field-dependent RA patterns over all $\beta$, which isolates $\beta$-independent symmetries. We also show the results of two different fitting schemes, in which the anomalous $C_1$ term either rotates with $\beta$ or is independent of $\beta$. In the first scheme, labeled "Free $C_1$", we use Eq. (8), which includes a fixed crystallographic EQ contribution, a $\beta$-dependent MD contribution, and an anomalous $\beta$-dependent $C_1$ ED contribution. As shown by Fig. 2(a) and Fig. S3, the fits are excellent, and as a result, the summation of the field-dependent fits matches the data well, as shown by the black curve in Fig. 2(b). In the second scheme, labeled "Fixed $C_1$", we first determine the $\beta$-independent EQ and anomalous $C_1$ ED tensor elements by fitting the zero-field RA pattern in Fig. 1(c) inset with Eq. (1). We then fit the 370 mT data by coherently adding the $\beta$-dependent MD term to the fixed EQ and ED terms. As shown by the red curve in Fig. 2(b), this fitting scheme imparts a noticeable $C_1$ dependence in the summation over $\beta$, which does not fit the data well. We can therefore conclude that the anomalous $C_1$ term rotates with $\beta$.

## VI. Fitting RA data by scaling the MD contribution

As discussed in the main text, another possible explanation we examined for the field-dependent SHG data is that the stacking order is altered to be $++++$ near the sample surface. In this scenario, we expect that all RA patterns can be described by only two terms: $4/m$ EQ and a magnetization-dependent $2'/m'$ MD SHG. Furthermore, there should be a perfect mapping from the high-field to the zero-field case by simply changing the MD tensor by a complex scale factor. To test this, we first fit the zero- (high-) field data by itself, then attempted to fit the high- (zero-) field data only by scaling the MD contribution to account for the different magnetization. The results of this exercise are shown by the solid black lines in Fig. S4. While the zero- and high-field patterns are qualitatively similar, there are clear discrepancies between the black curves and the data, which is further evidence against the existence of an anomalous ferromagnetic stacking in part of the sample. On the other hand, the data fit well to the model in Section III and IV, as shown by the shaded areas.

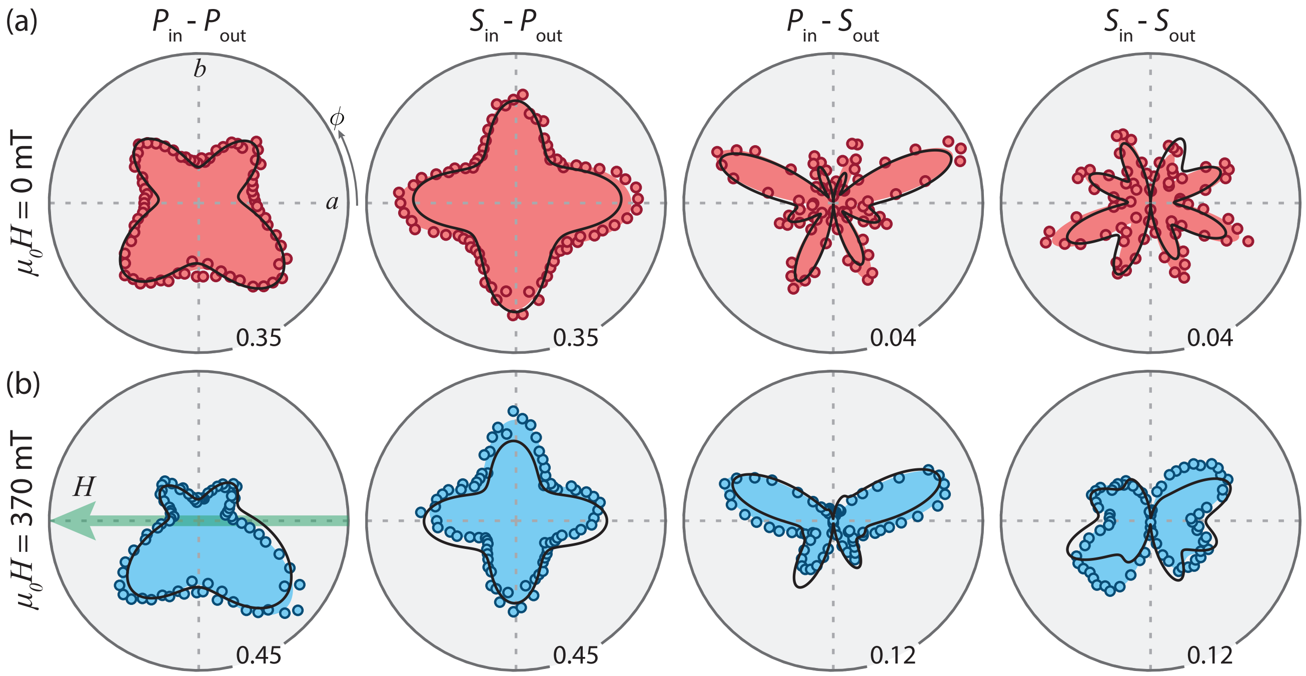


FIG. S4. RA-SHG polar plots for all four polarization geometries measured at 80 K with (a) 0 mT and (b) 370 mT in-plane magnetic field along $[\bar{1}00]$. Note that the plots have different radial axis scales, which are indicated by the numbers on the outer boundary of the plot. The shaded areas are simultaneous fits of 0 mT and 370 mT data within each polarization geometry assuming there is a magnetic surface ED SHG term. The solid black lines are fits using the magnetization scaling scheme described in the text.

### VII. SHG evidence for $a$-$b$ symmetry breaking and twinning

As we discussed in the main text and Section V, we can expose $\beta$-independent symmetries by summing the RA-SHG patterns over magnetic field angles $\beta$ from 0 to $2\pi$. A clear twofold symmetry is observed in Fig. 2(b), signifying a different magnetic field response along $a$ and $b$. This symmetry persists at 220 K [Fig. S5(a)], though with a slightly more subtle distortion due to the weakened magnetic term. We do not observe appreciable twofold distortions in the EQ SHG response at room temperature [Fig. S5(b)]. There are two potential explanations for these data. The first is pseudospin-lattice coupling, which creates a uniaxial anisotropy in-plane along the direction of the layer magnetization. The effect of pseudospin-lattice coupling shows itself in the intermediate magnetic field range [11, 12], where the applied field is comparable to the critical field of the metamagnetic transition, as seen, for example, in the twofold symmetry in the magnetic field direction dependence of out-of-plane anisotropic magnetoresistance [13, 14]. This metamagnetic transition and anisotropy are strongly dependent on temperature [11]. At 80 K, the magnetization becomes fully saturated for all field directions above $\sim$0.3 T, while at 220 K, the saturation is achieved by $\sim$0.1 T. Above these fields, one expects a return to $C_4$ symmetry in the field direction dependence, which should be the case for our SHG experiments. As a result, the observed twofold symmetry points instead to an alternative explanation: the existence of a distortion below tetragonal symmetry that exists above $T_N$. This is consistent with the observation in Fig. 4c that the order parameter only changes by 0° or 180° upon thermal cycling in zero field. However, the distortion is subtle enough that it is not detected by RA-SHG above $T_N$.

Figure S6 shows the magnetic field response from two different SHG domains with $C_1$ order parameters that are rotated by 90° at zero field. In the first region (domain A) with $\beta = 0°$ (top left), the $P_{\text{in}}$-$S_{\text{out}}$ pattern shows two lobes of equal intensity. When the field is rotated to $\beta = 90°$, however, we only observe a single strong lobe (bottom left). This is the same behavior that was found in Fig. 2(a). In contrast, for domain B, the field-direction-dependent response switches; one strong lobe is seen for $\beta = 0°$, while two are present for $\beta = 90°$. By inspecting the patterns, we see that region B is related to A by an interchange of the $a$ and $b$ axes. In other words, the SHG domains related by relative surface magnetizations of 90° are $a$-$b$ twins, with locked magnetic and crystallographic ordering.

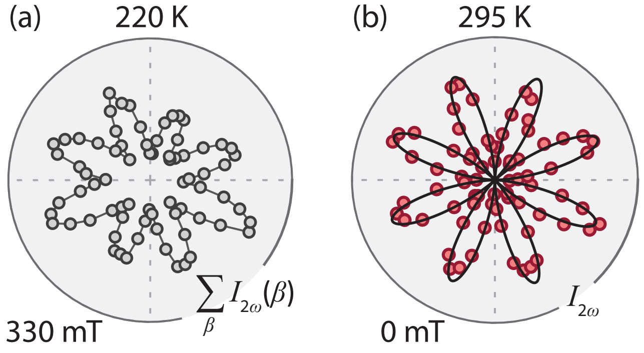


FIG. S5. (a) Plot of $P_{\text{in}}$-$S_{\text{out}}$ RA-SHG patterns summed over $\beta$, where $\beta$ runs from 0° to 315° in 45° increments. (b) RA-SHG intensity pattern for $P_{\text{in}}$-$S_{\text{out}}$ at 295 K. The solid black line is a fit to $4/m$ EQ SHG.

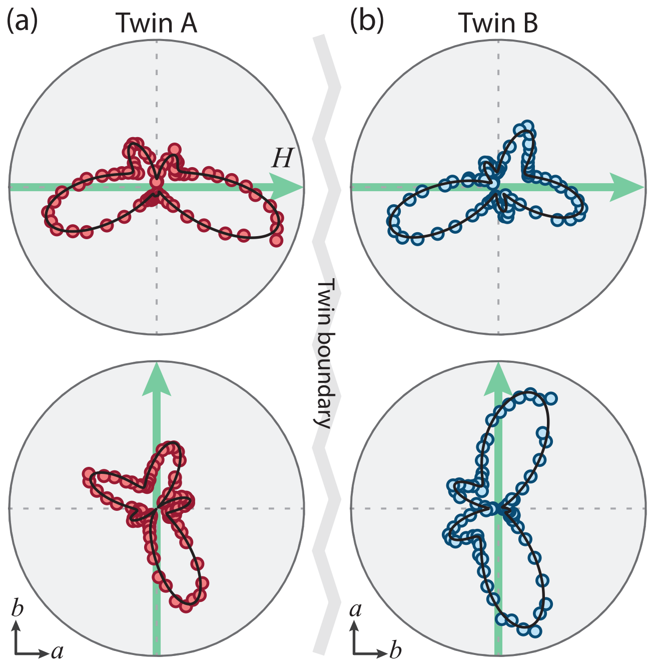


FIG. S6. RA-SHG intensity pattern at 80 K in $P_{\text{in}}$-$S_{\text{out}}$ geometry with 330 mT magnetic field applied along [100] (top) and [010] (bottom) for (a) twin region A and (b) twin region B. The two regions are crystallographic twins where the $a$ and $b$ axes have been interchanged.

[1] X. Chen, J. L. Schmehr, Z. Islam, Z. Porter, E. Zoghlin, K. Finkelstein, J. P. C. Ruff, and S. D. Wilson, Unidirectional spin density wave state in metallic $(Sr_{1-x}La_x)_2IrO_4$, Nat. Commun. **9**, 103 (2018).

[2] L. Zhao, D. H. Torchinsky, H. Chu, V. Ivanov, R. Lifshitz, R. Flint, T. Qi, G. Cao, and D. Hsieh, Evidence of an odd-parity hidden order in a spin-orbit coupled correlated iridate, Nat. Phys. **12**, 32 (2015).

[3] N. H. Sung, H. Gretarsson, D. Proepper, J. Porras, M. Le Tacon, A. V. Boris, B. Keimer, and B. J. Kim, Crystal growth and intrinsic magnetic behaviour of $Sr_2IrO_4$, Philos. Mag. **96**, 413 (2016).

[4] J. W. Harter, L. Niu, A. J. Woss, and D. Hsieh, High-speed measurement of rotational anisotropy nonlinear optical harmonic generation using position-sensitive detection, Opt. Lett. **40**, 4671 (2015).

[5] S. Di Matteo and M. R. Norman, Magnetic ground state of $Sr_2IrO_4$ and implications for second-harmonic generation, Phys. Rev. B **94**, 075148 (2016).

[6] D. H. Torchinsky, H. Chu, L. Zhao, N. B. Perkins, Y. Sizyuk, T. Qi, G. Cao, and D. Hsieh, Structural distortion-induced magnetoelastic locking in $Sr_2IrO_4$ revealed through nonlinear optical harmonic generation, Phys. Rev. Lett. **114**, 096404 (2015).

[7] R. R. Birss, *Symmetry and magnetism* (North-Holland Pub. Co., 1964).

[8] M. Fiebig, V. V. Pavlov, and R. V. Pisarev, Second-harmonic generation as a tool for studying electronic and magnetic structures of crystals: review, J. Opt. Soc. Am. B, JOSAB **22**, 96 (2005).

[9] A. Kirilyuk and T. Rasing, enMagnetization-induced-second-harmonic generation from surfaces and interfaces, J. Opt. Soc. Am. B **22**, 148 (2005).

[10] B. J. Kim, H. Ohsumi, T. Komesu, S. Sakai, T. Morita, H. Takagi, and T. Arima, Phase-sensitive observation of a spin-orbital Mott state in $Sr_2IrO_4$, Science **323**, 1329 (2009).

[11] J. Porras, J. Bertinshaw, H. Liu, G. Khaliullin, N. H. Sung, J.-W. Kim, S. Francoual, P. Steffens, G. Deng, M. M. Sala, A. Efimenko, A. Said, D. Casa, X. Huang, T. Gog, J. Kim, B. Keimer, and B. J. Kim, Pseudospin-lattice coupling in the spin-orbit mott insulator $Sr_2IrO_4$, Phys. Rev. B **99**, 085125 (2019).

[12] H. Liu and G. Khaliullin, Pseudo-Jahn-Teller effect and magnetoelastic coupling in spin-orbit Mott insulators, Phys. Rev. Lett. **122**, 057203 (2019).

[13] C. Wang, H. Seinige, G. Cao, J.-S. Zhou, J. B. Goodenough, and M. Tsoi, Anisotropic magnetoresistance in antiferromagnetic $Sr_2IrO_4$, Phys. Rev. X **4**, 041034 (2014).

[14] H. Wang, C. Lu, J. Chen, Y. Liu, S. L. Yuan, S.-W. Cheong, S. Dong, and J.-M. Liu, Giant anisotropic magnetoresistance and nonvolatile memory in canted antiferromagnet $Sr_2IrO_4$, Nat. Commun. **10**, 2280 (2019).
